# Supplementary material for: Mitigating Cold-start Forecasting using Cold Causal Demand Forecasting Model
Source: arXiv:2306.09261 source file (2023-06-15)
Supplement: Supplementary file 1 [file 7-appendix.tex]

%\newpage
%\pagebreak

\appendix
